# Supplementary material for: Persistent detwinning of iron pnictides by small magnetic fields
Source: arXiv:1408.6666 source file (2014-08-28)
Supplement: Supplementary file 1 [file Supplement.pdf]

# Persistent detwinning of iron pnictides by small magnetic fields: Supplementary Information

S. Zapf,[1] C. Stingl,[2] K. Post,[3] J. Maiwald,[2,4] N. Bach,[2] I. Pietsch,[2] D. Neubauer,[1] A. Löhle,[1] C. Clauss,[1] S. Jiang,[1] H. S. Jeevan,[2,5] D. Basov,[3] P. Gegenwart,[2,4] and M. Dressel[1]

[1] *1. Physikalisches Institut, Universität Stuttgart, Pfaffenwaldring 57, 70550 Stuttgart, Germany*
[2] *I. Physikalisches Institut, Universität Göttingen, Friedrich-Hund-Platz 1, 37077 Göttingen, Germany*
[3] *Department of Physics, University of San Diego, 9500 Gilman Drive, 92093 La Jolla, California, USA*
[4] *Experimentalphysik VI, Universität Augsburg, Universitätsstraße 1, 86135 Augsburg, Germany*
[5] *Department of Physics, PESITM, Sagar Road, 577204 Shimoga, India*

## I. METHODS

$EuFe_2As_2$ single crystals were grown by using the self-flux method as described in Ref. 1. Characterization by energy-dispersive x-ray analysis and x-ray diffraction confirms the composition and structure, respectively. The sample was then oriented with a Laue camera and (if needed) cut along the $[110]_T$-direction using spark erosion. Typical dimensions after cutting were $2 \times 1 \times 0.1\,\mathrm{mm}^3$.

DC-transport measurements were performed with a standard Physical Property Measurement System (PPMS) in the Montgomery geometry; magnetostriction and thermal expansion measurements with a miniaturized, high-resolution capacitive dilatometer[2] installed in a PPMS. The optical reflectivity was investigated by Fourier-transform spectroscopy in the far-infrared frequency range (100-700 $\mathrm{cm}^{-1}$), using a magnetospectroscopic apparatus as described in Ref. 3. Magnetization measurements were carried out in a SQUID-magnetometer.

Using the dilatometer, a spring force of 3 N is necessarily exerted on the sample, corresponding to a uniaxial pressure of about 13.5 bar (in the *ab*-plane). While this is not enough to fully detwin the sample[4], a non-linear influence on the twin configuration cannot be excluded (see section III). All other measurements were performed with mounting techniques that minimize the external stress on the sample: for resistivity measurements, the sample was glued on only one corner, leaving it free to contract and expand during the measurements. Furthermore, the Montgomery geometry minimizes the contact area and therefore stress and strain effects induced by the contacts. For optics, the sample was mounted on a copper cone. This avoids not only back-reflections from the sample holder, but also minimizes the glued area. For the magnetization measurements, the sample was fixed between two stripes of plastic foil by wrapping Teflon tape around them.

## II. COMPARISON MEASUREMENTS

In our main text, we present a mechanism for detwinning $EuFe_2As_2$ single crystals by applying small magnetic fields along the orthorhombic axes, *i.e.* the $[110]_T$-direction. In order to verify the effect, we have repeated all measurements on $EuFe_2As_2$ with $H \parallel [100]_T$, *i.e.* with the magnetic field at a 45° angle to the easy axes of the $Eu^{2+}$ magnetic moments in *both* twin variants. In this case, no twin is favored and thus, no detwinning should appear (limited by our accuracy of aligning the crystal perfectly along the $[100]_T$-direction). Additionally, comparison measurements were performed on $BaFe_2As_2$ single crystals with $H \parallel [110]_T$.

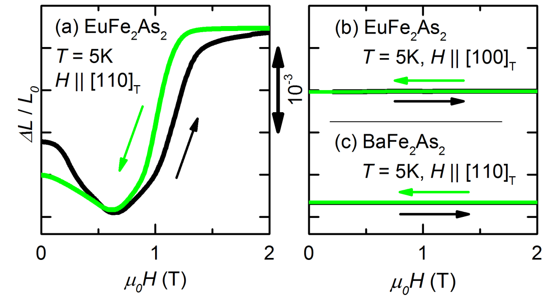


FIG. S1. Magnetostriction of $EuFe_2As_2$ and $BaFe_2As_2$ at $T = 5\,\mathrm{K}$ for different magnetic field directions. All plots share the same scale. (a) $EuFe_2As_2$, $H \parallel [110]_T$, (b) $EuFe_2As_2$, $H \parallel [100]_T$, and (c) $BaFe_2As_2$, $H \parallel [110]_T$. Detwinning is only observed for $EuFe_2As_2$ when the field is parallel to the crystal's orthorhombic axes.

Figure S1a shows the magnetostriction of $EuFe_2As_2$ with the external magnetic field $H \parallel [110]_T$. As discussed in the main text, small magnetic fields of $\sim 1\,\mathrm{T}$ influence the elongation of the $EuFe_2As_2$ sample drastically. However, if the field is applied along the $[100]_T$-direction (see Fig. S1b), no comparable change is observed, just as for $BaFe_2As_2$ (see Fig. S1c). The same is true for the magneto-optical measurements (see Fig. S2). Up to 1 T, the reflectivity does neither show any magnetic field induced anisotropy for $BaFe_2As_2$ with $H \parallel [110]_T$, nor for $EuFe_2As_2$ with $H \parallel [100]_T$. Furthermore, magnetization

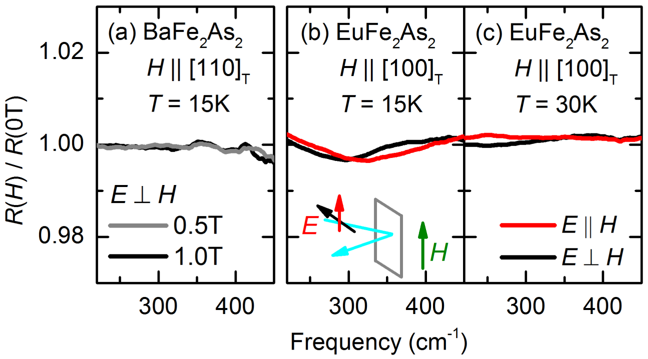


FIG. S2. Frequency dependent relative reflectivities of $BaFe_2As_2$ ($T$ =15 K) and $EuFe_2As_2$ ($T$ =15 K, 30 K) for different magnetic field directions. Relative reflectivities of (a) $BaFe_2As_2$ with $H \parallel [110]_T$ ($T$ =15 K) and (b,c) $EuFe_2As_2$ with $H \parallel [100]_T$ ((b) $T$ =15 K and (c) 30 K) do not show magnetic field induced anisotropy.

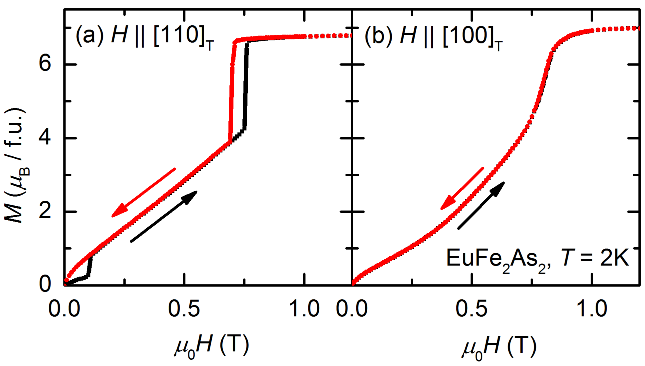


FIG. S3. Field dependent magnetization of $EuFe_2As_2$ at $T$ =2 K for different magnetic field directions.(a) $H \parallel [110]_T$ and (b) $H \parallel [100]_T$. Irreversible behavior is only observed, when the field is parallel to the crystal's orthorhombic axes.

measurements on $EuFe_2As_2$ (see Fig. S3) exhibit strong irreversible behavior induced by domain dynamics only for $H \parallel [110]_T$, but not for $H \parallel [100]_T$.

In summary, our reference measurements provide evidence that the observed effects which are subject of our report must be related *(i)* to a redistribution of twins and *(ii)* to the presence of $Eu^{2+}$ moments.

## III. THERMAL EXPANSION AND MAGNETOSTRICTION

Thermal expansion measurements directly probe the length changes of a sample and can thus yield quantitative information about the twin distribution. In Fig. S4, we compare our results with the temperature dependent orthorhombic lattice parameters $a(T)$ and $b(T)$, measured by Tegel *et al.* with x-ray diffraction[5]. Assuming a temperature independent fraction $n$ of twins with $b \parallel H$, the mean length of a unit cell in field direction follows as

$$\bar{L} = n \cdot b(T) + (1-n) \cdot a(T). \quad (1)$$

The relative length change compared to $a_T$ (the tetragonal lattice constant at 300 K) then reads as:

$$\frac{\Delta L}{L_0} = \frac{\bar{L} - a_T}{a_T} \quad . \quad (2)$$

By setting $n = 66\%$, we can reproduce the ZFC curve in Fig. S4 reasonably well, indicating that the sample is already partially detwinned without the application of any external magnetic field. We ascribe this to the uniaxial pressure from the dilatometer (see section I), which favors twins with $b \parallel \Delta L$, as soon as the sample is cooled below $T_{s,SDW}$. Nevertheless, the twin configuration can be changed to $n = 70\%$ by field treatment, causing substantial length changes of the order of $\sim 10^{-3}$.

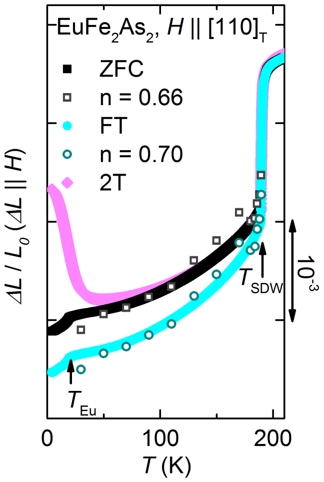


FIG. S4. Thermal expanison measurements on $EuFe_2As_2$ with $\Delta L \parallel H \parallel [110]_T$, together with calculated twin domain ratios. Thermal expansion after FT with 2 T at 4 K (cyan solid dots) and ZFC (black solid squares), as well as under an applied magnetic field of 2 T (magenta solid diamonds). Curves are shifted to merge at 300 K. The open symbols present sample lengths calculated from x-ray data[5] by assuming temperature independent twin domain ratios, as indicated $n = 66\,\%$ and $70\,\%$.

Magnetic fields around 1 T, which detwin the crystal with its $a$-axis along $H$, counteract the induced dilatometer pressure. Nevertheless, we are still able to observe at low temperatures a distinct increase of the sample length (see Fig. S1, Fig. S4, and Fig. S5). However, with increasing temperature, the Zeeman energy must compete with thermal energy and the magnetization in the $Eu^{2+}$ system at a certain external field decreases. As a consequence, the thermal expanison curve with applied magnetic field approaches the 0 T curve at elevated temperatures (see Fig. S4). In summary, although the dilatometer induces a pressure along the direction of $H$ and measured $\Delta L$, we are able to observe a magnetic field

induced decrease and increase of the sample length, consistent with our interpretations of magnetic detwinning.

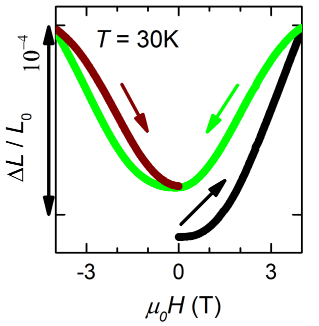


FIG. S5. Magnetostriction $\Delta L(H)/L_0$ of ZFC $EuFe_2As_2$ ($H \parallel [110]_T$) at 30 K for increasing (black, brown) and decreasing (green) $H$.

Our observations have a remarkable parallel to the field-induced deformation in magnetic shape memory alloys such as Fe-Pd[6] or Ni-Mn-Ga[7]. In these systems, below a structural phase transition from austenite to martensite, magnetic fields comparable to ours can induce large strains of several percent by twin boundary movement. However, the magnetic ordering in magnetic shape memory systems is usually ferromagnetic and they do not show the complex elongation-contraction sequence which we find in $EuFe_2As_2$.

## IV. PHONON DYNAMICS

According to theoretical and experimental studies, the phonon modes in $BaFe_2As_2$ are very sensitive to the structural transition[8–10]. In particular, the Fe-As mode at $257\,cm^{-1}$ splits in the orthorhombic phase, with the dominating contribution at lower frequencies corresponding to the crystallographic $b$-axis. A strongly asymmetric lineshape indicates that the vibrational feature couples to the free electron response.

In Fig. S6 we compare the 15 K optical conductivity of twinned $EuFe_2As_2$ for two orthogonal polarizations in the spectral range of the Fe-As vibration. In the virgin state, the mode is isotropic and agrees with previous observations[11] of the Fe-As vibration at $\sim 260\,cm^{-1}$. In the detwinned state at 1 T, the response becomes anisotropic. We calculate the optical conductivity via a Kramers-Kronig transformation, using 0 T data for an appropriate extrapolation. Although we also observe an asymmetric lineshape of the dominant contribution, we can not resolve a splitting of the phonon. (The authors of Ref. 8 could achieve a better signal-to-noise ratio as they did not use any polarizer in a zero-field cryostat.) However, we clearly resolve that the conductivity along the $b$-direction ($E \perp H$) is reduced, but the oscillator strength of the Fe-As mode becomes considerably enhanced. This observation is consistent with the results for $BaFe_2As_2$. For $E \parallel H$, the $260\,cm^{-1}$ mode can still be identified, albeit its intensity is strongly reduced. We attribute its presence to the imperfect polarizer and the improper alignment of polarizer and sample with respect to the external magnetic field. Since the phonon is rather strong, this allows the Fe-As mode to show up also in the perpendicular direction and reduces the intensity for the polarization $E \perp H$, observed also for mechanically detwinned $BaFe_2As_2$[9]. Nevertheless, the intensity changes of the phonon mode, visible also in Fig. 3 of the main text, fully agree with our model and strongly support the magnetic detwinning.

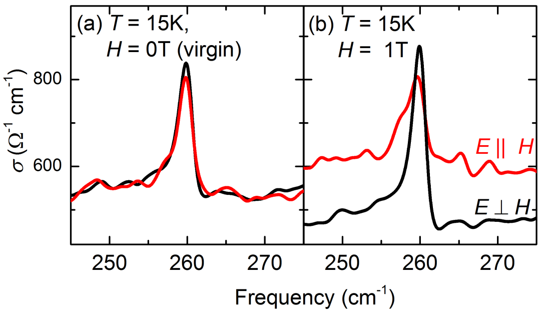


FIG. S6. Polarization dependent optical conductivity of $EuFe_2As_2$ around the Fe-As phonon mode at $\sim 260\,cm^{-1}$ for 15 K with and without magnetic field. (a) 0 T (virgin), (b) 1 T ($H \parallel [110]_T$, resolution $1\,cm^{-1}$). In the magnetic field, the oscillator strength of the phonon is enhanced for the polarization direction with lower conductivity ($E \perp H$, black) and reduced for that with higher conductivity ($E \parallel H$, red).

## V. MAGNETIZATION

Figure S7 displays the temperature dependent magnetization of $EuFe_2As_2$ with $H \parallel [110]_T$. While $M(T)$ results at lowest fields from a superposition of antiferromagnetic susceptibilities parallel and perpendicular to the easy axis (see Fig. S7a), for $H > H_1$ and after FT, twins with $b \parallel H$ are dominant and thus $M(T)$ is governed by the perpendicular susceptibility (see Fig. S7b,d). Above $H_{SF}$, field enforced ferromagnetism sets in (see Fig. S7c).

## VI. PHENOMENOLOGICAL MODEL

### A. Antiferromagnetism

In order to qualitatively describe the behavior of the $Eu^{2+}$ spins in an external magnetic field $H$, we consider a simple model of antiferromagnetically aligned spins with coupling constant $J$ under the influence of an external magnetic field $H$ and a magneto-crystalline anisotropy $\Delta$ (at $T = 0\,K$). In a twinned crystal, two domain types appear, one with the (easy) $a$-axis perpendicular (type $B_{\parallel}$)

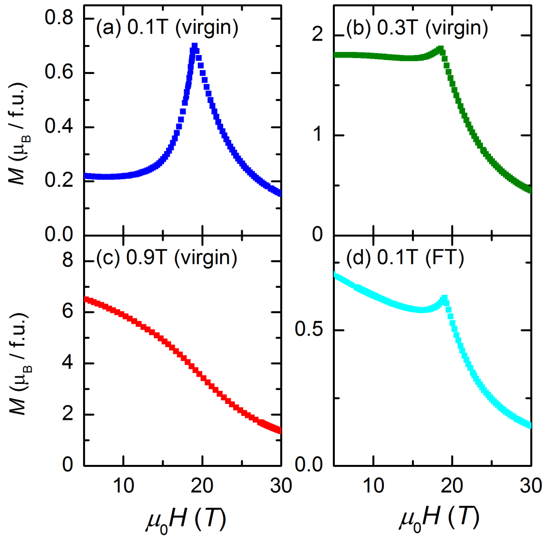


FIG. S7. Temperature dependent magnetization for $EuFe_2As_2$ at certain magnetic fields $H \parallel [110]_T$ with and without field treatment. (a) 0.1 T (virgin), (b) 0.3 T (virgin), (c) 0.9 T (virgin), and (d) 0.1 T (FT).

and one with it parallel (type $A_{||}$) to $H$.

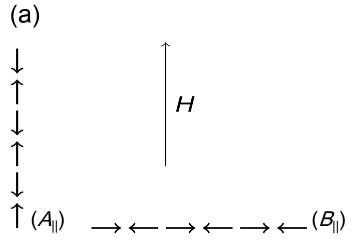


FIG. S8. Phenomenological model. (a) Ground state antiferromagnetic ordering of twins $A_{||}$ and $B_{||}$ with respect to an external magnetic field $H$. (b) Defined angles between $H$ and spins.

The simplest form for the energy is then given by[12,13]:

$$E = -2M\mu_0 H(\cos\theta + \cos\varphi) + JM^2\cos(\theta+\varphi) - \frac{1}{2}\Delta \begin{cases} \sin^2\theta + \sin^2\varphi & (B_{||}) \\ \cos^2\theta + \cos^2\varphi & (A_{||}) \end{cases}, \quad (3)$$

where $\theta$ and $\varphi$ are the angles between spins and magnetic field (see Fig. S8) and $E_0 = -JM^2 - \Delta$ is the 0 T ground state energy. Minimizing the energy for $\theta = \varphi$ yields:

$$E_{\text{min}}^{B_{||}} = E_0 - \frac{M^2(\mu_0 H)^2}{2JM^2 + \Delta} \quad (4)$$

$$E_{\text{min}}^{A_{||}} = E_0 + \Delta - \frac{M^2(\mu_0 H)^2}{2JM^2 - \Delta} \quad (5)$$

Equations (4) and (5) are plotted in Fig. 4e of the main text. As we describe there in detail, the simple model can qualitatively explain the two-step detwinning process observed in our measurements.

### B. Detwinning fraction

The question remains why the crystal does not get completely detwinned at $H_1$ (otherwise no spin flip would be visible at higher fields, as no domains of type $A_{||}$ would be left). As our techniques are non-local probes, we can only speculate about this issue. One possible influence could be the three-dimensional nature of the A-type antiferromagnetism, as presented in Fig. S9. Within one layer, $Eu^{2+}$ spins of next-nearest structural domains can be aligned after ZFC parallel (see Fig. S9a,b) or antiparallel (see Fig. S9c,d). The reorientation of the intermediate domain at $H_1$ will be less favorable for the latter case, as some kind of magnetic domain wall will be left.

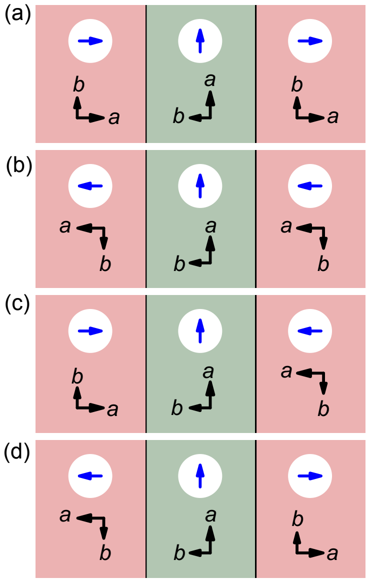


FIG. S9. Considering the three-dimensionality of A-type antiferromagnetism could explain, why the crystal gets not completely detwinned at $H_1$. Within one layer, $Eu^{2+}$ spins (blue) of next-nearest structural domains can be aligned (a,b) parallel or (c,d) antiparallel. The reorientation of the intermediate domain will be less favorable for the latter case.

## VII. COOLING PROCEDURE

In order to observe the low-field magnetic detwinning, the sample needs to be cooled in zero field through $T_{\text{s,SDW}}$, as already described in the main text. Here we present additional data which prove the importance of a well-defined cooling procedure.

As presented in Fig. 3 of the main text, the low-field detwinning process leads to irreversibilities in the field dependent magnetization. However, those are only visible in the first field cycling after zero-field cooling. This is demonstrated in Fig. S10, showing an additional field sweep.

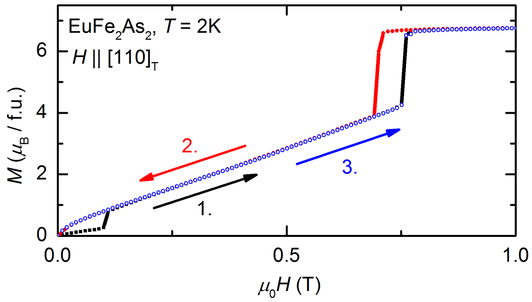


FIG. S10. Field dependent magnetization of $EuFe_2As_2$ at $T = 2\,K$ for $H \parallel [110]_T$. Irreversible behavior at low fields ($\sim 0.1\,T$) is only observed in the first field cycling after ZFC.

Moreover, reflectivity data presented in Fig. S11 evidence that any persistence gets removed at $T_{s,SDW}$: after the crystal got persistently detwinned at 30 K, a small anisotropy is still detectable when heating up to 100 K and 180 K. However, if the crystal was once heated above the structural and spin-density-wave transition ($T_{s,SDW} = 190\,K$) and cooled down afterwards in zero field, this anisotropy has completely vanished (see Fig. S11d).

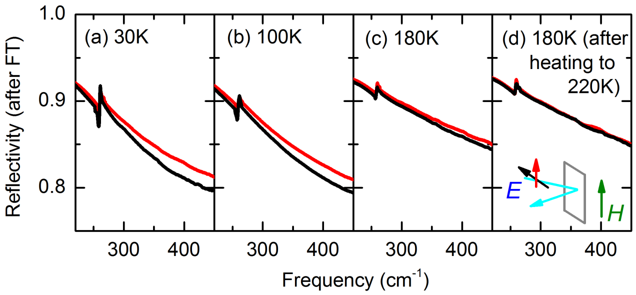


FIG. S11. Frequency dependent reflectivity of $EuFe_2As_2$ after field treatment at $T = 30\,K$ with 1 T ($H \parallel [110]_T$) for (a) 30 K, (b) 100 K and (c) 180 K. Although the magnetic field is switched off during the measurement, the reflectivity along the orthorhombic axes is anisotropic. (d) After the crystal was heated to 220 K (well above $T_{s,SDW}$) and cooled down again to 180 K, any anisotropy disappeared.


[1] H. S. Jeevan, D. Kasinathan, H. Rosner, and P. Gegenwart, Phys. Rev. B **83**, 054511 (2011).

[2] R. Küchler, T. Bauer, M. Brando and F. Steglich, Rev. Sci. Instr. **83**, 095102 (2012).

[3] A. D. LaForge, A. Frenzel, B. C. Pursley, Tao Lin, Xinfei Liu, Jing Shi, and D. N. Basov, Phys. Rev. B **81**, 125120 (2010).

[4] I. R. Fisher, L. Degiorgi, and Z. X. Shen, Rep. Prog. Phys. **74**, 124506 (2011).

[5] M. Tegel, M. Rotter, V. Weiß, F. M. Schappacher, R. Pöttgen, and D. Johrendt, J. Phys. Condens. Mat. **20**, 452201 (2008).

[6] R. D. James and M. Wuttig, Phil. Mag. A **77**, 1273 (1998).

[7] A. Sozinov, A. Likhachev, N. Lanska, and K. Ullakko, Appl. Phys. Lett.**80**, 1746 (2002).

[8] A. A. Schafgans, B. C. Pursley, A. D. LaForge, A. S. Sefat, D. Mandrus, and D. N. Basov, Phys. Rev. B **84**, 052501 (2011).

[9] M. Nakajima, T. Liang, S. Ishida, Y. Tomioka, K. Kihou, C. H. Lee, A. Iyo, H. Eisaki, T. Kakeshita, T. Ito, and S. Uchida, PNAS **108**, 12238 (2011).

[10] A. Akrap, J. J. Tu, L. J. Li, G. H. Cao, Z. A. Xu, and C. C. Homes, Phys. Rev. B **80**, 180502(R) (2009).

[11] D. Wu, N. Barišić, N. Drichko, S. Kaiser, A. Faridian, M. Dressel, S. Jiang, Z. Ren, L.J. Li, G.H. Cao, Z.A. Xu, H.S. Jeevan, and P. Gegenwart, Phys. Rev. B **79**, 155103 (2009).

[12] S. Blundell, *Magnetism in Condensed Matter.* (Oxford University Press Inc., New York, 2001).

[13] M. Getzlaff, *Fundamentals of Magnetism.* (Springer, Berlin, 2008).
